# Supplementary material for: Privacy Accounting and Quality Control in the Sage Differentially Private ML Platform
Source: arXiv:1909.01502 source file (2019-09-06)
Supplement: Supplementary file 1 [file classification-evaluation.tex]

\begin{table}
	\footnotesize
	\centering
	\begin{tabular}{l|cl}
		\hline
		{\bf Models:} & \multicolumn{2}{l}{{\bf Configuration:}} \\
		\hline
		\multirow{4}{1.3cm}{Logistic Regression ({\bf LR})} & DP Alg. & DP SGD from \cite{mcmahan2018general}, $(\e,\delta)$-DP\\
		\cline{2-3}
		& Config. & Learning rate: $0.1$, Epochs: 3 Batch: 512\\
		\cline{2-3}
		& Budgets & $\ed \in \{(1.0, 10^{-6}), (0.25, 10^{-6})\}$ \\
		\cline{2-3}
		& Targets & Accuracy $\in [0.74, 0.78]$  \\
		\hline
		\hline
		\multirow{5}{1.3cm}{Neural Network ({\bf NN})} & DP Alg. & DP SGD from \cite{mcmahan2018general}, $\ed$-DP\\
		\cline{2-3}
        &         & ReLU, 2 hidden layers (1024/32 nodes) \\
		& Config. & Learning rate: 0.01, Epochs: 5\\
		&            & Batch: 1024 \\
		\cline{2-3}
		& Budgets & $\ed \in \{(1.0,10^{-6}),(0.25,10^{-6})\}$ \\
		\cline{2-3}
		& Targets & Accuracy $\in [0.74, 0.78]$  \\
		\hline
		\end{tabular}
	\caption{{{\bf Experimental Criteo Classification Training Pipelines.}
	}}
	\vspace{-1cm}
	\label{t:private-criteo-classification-models}
\end{table}

We evaluate \sysname using the publicly released Criteo click prediction dataset~\cite{criteoKaggle}.
This is a binary classification dataset where each example is an ad impression and the goal is to predict if a user will click on the ad.
The dataset is a sample collected over 7 days and consists of 45 million observations with 39 features per observation.
Each observation has 13 numeric features and 26 categorical features some of which with very high cardinalities (> 1M).
The models consume the 13 numeric features as real values and the 26 categorical features using feature hashing~\cite{weinberger2009feature}.
We implement two predictive models training pipelines, a logistic regression (LR) and a neural network (DNN) using TensorFlow~\cite{abadi2016tensorflow} and the TensorFlow Privacy library~\cite{tensorflow-privacy}.
\T~\ref{t:private-criteo-classification-models} lists the configuration and hyperparameters for each model.
We use accuracy, the fraction of observations classified correctly, as the evaluation metric for this dataset and use the accuracy validator defined in~\ref{appendix:sla-tests:accuracy}.
74.3\% of the observations have the no-click label which we configure as the lower bound on the accuracy targets for both models.
As with the regression evalaution we hold out 100K data points for evaluation and use a 90\%::10\% train::test ratio; $\eta=0.05$; $\delta=10^{-6}$.

\begin{figure}[t]
	\centering
	\footnotesize
	\begin{subfigure}[t]{0.490\linewidth}
        \includegraphics[width=\linewidth]{results/linear_criteo_accuracy_classification_performance}
		\caption{{\bf LR Accuracy}}
		\label{fig:evaluation:impact-of-dp-on-model-accuracy-linear-classification}	
	\end{subfigure}
\begin{subfigure}[t]{0.490\linewidth}
        \includegraphics[width=\linewidth]{results/dnn_criteo_accuracy_classification_performance}
		\caption{{\bf NN Accuracy}}
		\label{fig:evaluation:impact-of-dp-on-model-accuracy-nn-classification}
	\end{subfigure}
	\vspace{-0.4cm}
	\caption{{\bf Impact of DP on Classification Models.}
	}  \label{fig:evaluation:impacts-of-dp-on-training-pipelines-classification}
	\vspace{-0.3cm}
\end{figure}

\subsection{Impact of Differential Privacy}

Figures~\ref{fig:evaluation:impact-of-dp-on-model-accuracy-linear-classification} and~\ref{fig:evaluation:impact-of-dp-on-model-accuracy-nn-classification} show the impact of differential privacy on the logistic regression and neural network respectively.
The figures show the amount of training data on the x axis and the accuracy of each model on the held out evaluation set on the y axis.
There is one line for the non-private model and lines for two different privacy budgets for each model.
The horizontal dashed line shows the performance of a naive baseline model that always predicts no-click.
\xxx{Naive punctuation}

All models outperform the baseline when trained on more than 100K data points.
This amounts to less than 1 hour of data collection.
\xxx{something about the LR}.

The private DNN models perform 1.8\%-2.0\% worse than the non private DNN.
This performance delta could be mitigated by training on a significanly larger amount of data or possibly by increasing the batch size.
Increasing the batch size will decrease the impact of each noise addition.
However, increasing the batch size may incur a significant penalty with respect to the training time.
The DNN models are trained using an NVIDIA V100 with 16GB of GPU memory.
Increasing the training batch size from 1024 to 2048 surpasses the amount of available GPU memory and incurs 2.5x overhead in training time using our hardware configuration which leads to the the private model to requiring nearly two days when training on the full training set.
This may cause operational problems because many companies have limits on the amount of time, 7 days for example, that may be spent training a single model.

\begin{figure}[t!]
	\begin{subfigure}{0.490\linewidth}
        \includegraphics[width=\linewidth]{results/linear_criteo_accuracy_classification_required_n_per_tau}
		\caption{{\bf LR \ACCEPT}}
		\label{f:criteo_lr_required_sample_complexity_classification}
	\end{subfigure}
	\begin{subfigure}{0.490\linewidth}
        \includegraphics[width=\linewidth]{results/dnn_criteo_accuracy_classification_required_n_per_tau}
		\caption{{\bf NN \ACCEPT}}
		\label{f:criteo_dnn_required_sample_complexity_classification}
	\end{subfigure}
	\vspace{-0.4cm}
	\caption{\footnotesize {\bf Sample Complexity of SLAed DP Validation.}
	}
	\label{fig:evaluation:data-needed-for-slaed-validation-classification}
	\vspace{-0.7cm}
\end{figure}

\subsection{Model Validation: Accept}
\F~\ref{fig:evaluation:data-needed-for-slaed-validation-classification} shows the amount of data required to meet different accuracy targets for the logistic regression and DNN models with $\epsilon=1$.
Both models require similar amounts of data for validation however the DNN is able to guarantee an accuracy of 77.5\% while the private linear model is only able to guarantee 77\% accuracy.
The DNN model requires more data to accept models with lower accuracy targets due to the fact that the DNN performns only slightly better than the baseline until trained on >100K points.
Model validation with \sysname's SLA incurs little overhead beyond the non-private and uncorrected SLA.
For Accuracy targets above 76\% there is also little to no overhead beyond the heuristic validation with no SLA either.

The amount of data required to validate the classification model is notable lower than to validate the regression model as shown in \F~\ref{fig:evaluation:data-needed-for-slaed-validation}.
This is due to two reasons.
First the loss validator defined in \S~\ref{appendix:sla-tests:loss} is much more conservative than the accuracy validator.
Second the magnitude of the loss is smaller than the magnitude of the loss is relatively smaller than the magnitude of the accuracy.
This means that the validator will require much more data to make a confident reject or accept decision.

\heading{Accept Violations}

\begin{table}
	\centering
	\footnotesize
	\begin{tabular}{|c|c|c|c|c|}
    \hline
    {\bf $\eta$ } & {\bf No SLA} & {\bf NP SLA} & {\bf UC DP SLA} & {\bf Sage SLA}\\
    \hline
    0.01 & 0.2267 & 0.0360 & 0.0365 & 0.0360\\
    \hline
    0.05 & 0.2267 & 0.0511 & 0.0512 & 0.0511\\
    \hline
    0.10 & 0.2267 & 0.0569 & 0.0575 & 0.0570\\
    \hline
	\end{tabular}
	\caption{\footnotesize {\bf Target Violation Rate of {\ACCEPT}ed Classification Models.}
		Violations are across LR and NN separately trained with \iterativetraining.}
	\label{tab:evaluation:acceptance-violation-rate-classification}
	\vspace{-0.7cm}
\end{table}

Models violate their accuracy targets 13.0\% of the time when using non-private heuristic TFX approach and 11.4\% of the time when using the private heuristic approach.
\xxx{FINISH THIS OUT}

\heading{Invalid Rejections}

\begin{wrapfigure}{r}{0.490\linewidth}
	\centering
	\vspace{-\intextsep}
	\hspace*{-\columnsep}
    \includegraphics[width=\linewidth]{results/linear_criteo_accuracy_classification_rejection_size}
	\vspace{-\intextsep}
	\caption{{\bf Samples to \REJECT.}}
	\label{fig:evaluation:data-needed-to-reject-classification}
	\vspace{-\intextsep}
\end{wrapfigure}
