# Supplementary material for: Privacy Accounting and Quality Control in the Sage Differentially Private ML Platform
Source: arXiv:1909.01502 source file (2019-09-06)
Supplement: Supplementary file 2 [file end-to-end-evaluation.tex]

This experiment is an end-to-end evaluation of \sysname with a workload consisting of a data stream and ML pipelines arriving over discrete time steps.
ML pipeline arrivals are generated from a gamma process with a fixed mean arrival rate, $m$, and fixed arrival rate variance, $\sigma^2$.
The arrivals are generated by sampling the time between job arrivals from a gamma distribution with shape and scale parameters $k$ and $\theta$.
$k$ and $\theta$ are derived from the $m$ and $\sigma^2$ with the following formula \dots
\xxx{To fill this in}.

We perform this experiment with two different configurations for data arrival.
The first is constant data arrival where the number of new examples arriving during each each discrete time period remains the same.
Under the second configuration, the number of new examples arriving is generated using the same gamma process procedure used to generate job arrivals but with a much higher mean arrival rate.

The pipeline workload is drawn from the XXX configurations of tasks and targets.
\xxx{The number of tasks and targets may change}.
We wish for the pipeline workload to be generated in such a way that pipelines with smaller sample complexities are more likely to be drawn then pipelines with larger sample complexities.
The possible piplines are split into 10 decile based buckets based on the pipelines non-private sample complexity.
We then use a zipf distribution to randomly choose a bucket.
The pipeline submitted is then chosen uniformly from the pipelines in the bucket.

We measure the mean and 90th percentile response time to compare the different strategies.
To accurately compare the strategies we need to measure the response times while the system is in a steady state.
To achieve a steady state we divide the experiment into thirds where each this is the amount of time expected to be required to accumulate 36M points (the size of the dataset).
When computing the response time we only consider the pipelines that arrive during the middle third.
