# Supplementary material for: Privacy Accounting and Quality Control in the Sage Differentially Private ML Platform
Source: arXiv:1909.01502 source file (2019-09-06)
Supplement: Supplementary file 3 [file multi-pipeline-example.tex]

\begin{lstlisting}[float,floatplacement=tbp,
    label={list:statistics_pipeline},
    language=Python,
    caption={{\bf Example Statistics Pipeline.}}]
def preprocessing_fn(inputs):
  outputs["dist_clipped"] = tf.clip_by_value(
    inputs["dist"], 0, 50) / 50
  return outputs

def mean_trainer_fn(hparams, schema, `\hl{epsilon})`:
  # TODO: There is an API mismatch here.
  # TODO: Show writing to a feature store.
  scale = epsilon / tft.size("dist_clipped")
  outputs["dp_dist_mean"] = tft.mean("dist_clipped")\
   + laplace(0.0, scale)
  return outputs

def mean_validator_fn(`\hl{epsilon})`:
  statistic_validator = \
    `\hl{sage.DPSumStatisticsValidator}`(
      model=mean_trainer.outputs.output,
      target=_MEAN_TARGET,
      `\hl{epsilon=epsilon, confidence=0.95, B=1}`)
  return statistic_validator

def var_trainer_fn(hparams, schema, `\hl{epsilon})`:
  scale = epsilon / tft.size("dist_clipped")
  outputs["dp_dist_var"] = tft.var("dist_clipped")\
   + laplace(0.0, scale)
  return outputs

def mean_validator_fn(`\hl{epsilon})`:
  statistic_validator = \
    `\hl{sage.DPSumStatisticsValidator}`(
      model=mean_trainer.outputs.output,
      target=_VAR_TARGET,
      `\hl{epsilon=epsilon, confidence=0.95, B=1}`)
  return statistic_validator
\end{lstlisting}

\begin{lstlisting}[float,floatplacement=tbp,
    label={list:regression_pipeline},
    language=Python,
    caption={{\bf Example Regression Pipeline.}}]
def preprocessing_fn(inputs):
  outputs["dist_clipped"] = tf.clip_by_value(
    inputs["dist"], 0, 50) / 50
  dist_z = `\sout{tft.scale\_to\_z\_score}``\hl{sage.scale\_to\_z\_score}`(
    dist_clipped, `\hl{mean=inputs["dp\_dist\_mean"],}`
    `\hl{var=inputs["dp\_dist\_var"]}`)
  duration_label = tf.clip_by_value(inputs["duration"],
    0, 7200) / 7200
  return {"duration": duration_label,
    "hour_of_day": inputs["hour_of_day"],
    "day_of_week": inputs["day_of_week"],
    "dist_z": dist_z,}
  return outputs

def trainer_fn(hparams, schema, `\hl{epsilon, delta})`: [...]
  feature_columns = [numeric_column("dist_z"),
    categorical_column("hour_of_day", num_buckets=24),
    categorical_column("day_of_week", num_buckets=7)]
  estimator = \
    `\sout{tf.estimator.DNNRegressor}``\hl{sage.DPDNNRegressor}`(
      config=run_config,
      feature_columns=feature_columns,
      dnn_hidden_units=hparams.hidden_units,
      `\hl{privacy\_budget=(epsilon, delta)}`)
  return tfx.executors.TrainingSpec(estimator,...)

def validator_fn(`\hl{epsilon})`:
  model_validator = \
    `\sout{tfx.components.ModelValidator}``\hl{sage.DPModelValidator}`(
      examples=examples_gen.outputs.output,
      model=trainer.outputs.output,
      metric_fn=_MSE_FN, target=_MSE_TARGET,
      `\hl{epsilon=epsilon, confidence=0.95, B=1}`)
  return model_validator
\end{lstlisting}

\begin{lstlisting}[float,floatplacement=tbp,
    label={list:classification_pipeline},
    language=Python,
    caption={{\bf Example Classification Pipeline.}}]
def preprocessing_fn(inputs):
  outputs["dist_clipped"] = tf.clip_by_value(
    inputs["dist"], 0, 50) / 50
  dist_z = `\sout{tft.scale\_to\_z\_score}``\hl{sage.scale\_to\_z\_score}`(
    dist_clipped, `\hl{mean=inputs["dp\_dist\_mean"],}`
    `\hl{var=inputs["dp\_dist\_var"]}`)
  tip_label = tf.cast(tf.greater(
    inputs["tip"] / inputs["total"], 0.2), tf.int64)
  return {"tip": tip_label,
    "hour_of_day": inputs["hour_of_day"],
    "day_of_week": inputs["day_of_week"],
    "dist_z": dist_z}
  return outputs

def trainer_fn(hparams, schema, `\hl{epsilon, delta})`: [...]
  feature_columns = [numeric_column("dist_z"),
    categorical_column("hour_of_day", num_buckets=24),
    categorical_column("day_of_week", num_buckets=7),
    crossed_column(["hour_of_day", "day_of_week"], num_buckets=
  estimator = \
    `\sout{tf.estimator.LinearClassifier}``\hl{sage.DPLinearClassifier}`(
      config=run_config,
      feature_columns=feature_columns,
      dnn_hidden_units=hparams.hidden_units,
      `\hl{privacy\_budget=(epsilon, delta)}`)
  return tfx.executors.TrainingSpec(estimator,...)

def validator_fn(`\hl{epsilon})`:
  model_validator = \
    `\sout{tfx.components.ModelValidator}``\hl{sage.DPModelValidator}`(
      examples=examples_gen.outputs.output,
      model=trainer.outputs.output,
      metric_fn=`\sout{\_LOG\_LOSS\_FN}``\hl{\_CLIPPED\_LOG\_LOSS\_FN}`,
      target=_LOG_LOSS_TARGET,
      `\hl{epsilon=epsilon, confidence=0.95, B=1}`)
  return model_validator

\end{lstlisting}

\L~\ref{list:statistics_pipeline}, \L~\ref{list:regression_pipeline}, and \L~\ref{list:classification_pipeline} show three example \sysname pipelines processing the New York City Yellow Cab dataset~\cite{yellowCabData}.
Each pipeline is composed of three stages:preprocessing, training, and validation.
The first pipeline, \L~\ref{list:statistics_pipeline}, computes the mean and variance of the distance of each cab ride which will later be used for standardization.
The second pipeline trains a regression model to predict the duration of each ride.
The final pipeline trains a classification model to predict if each rider will give a large tip (> 20\%).

All pipelines are composed of three stages.
The first stage is responsible for any data independent preprocessing that must be performed before computing the model.
The second stage actually computes the model or statistic.
The final stage validates that the model meets its accuracy target.
If validation fails then the pipeline is restarted with either more data or a larger privacy budget allocation.

\L~\ref{list:statistics_pipeline} shows two pipelines that compute two statistics, the variance and mean of the cab ride distance.
These statistics will be used in later pipelines to performn standarization; a common feature engineering technique for numerical data.
Both statistic pipelines share a preprocessing function that clips the duration to be in a predefined range, $[0\text{km}, 50\text{km}]$, and then scaled to be between 0 and 1.
The duration value must have a known range to compute the sensitivity to add the differentially private noise.
The train function for each pipeline computes mean and variance using standard approaches and then sanitzes the result with a draw from an appropriately scaled laplace distribution.
The final stage in the pipeline, validation, validates that both statistics meet their targets using the DPSumValidator which implements the validation protocol defined in \S~\ref{appendix:sum-validation}.

\L~\ref{list:regression_pipeline} and \L~\ref{list:classification_pipeline} show two pipelines for training predictive models.
Both pipelines consist of similar preprocessing, training, and validation steps.
The preprocessing functions clip the distance into a predefined range and then uses the mean and variance computed in \L~\ref{list:statistics_pipeline} to perform standardization.
The function must also clip the regression label, duration, into a predefined range so that \sysname can compute the sensitivity of the validation function.
The train function switches the call to the non-private regressor with the DP implementation, which in \sysname is a simple wrapper around Tensorflow's DP SGD-based optimizer.
The validation function invokes \sysname's DP loss validator.
One notable change in \L~\ref{list:classification_pipeline} is that \sysname must compute a clipped logistic loss value to be in the range $[0, 1]$ because logistic loss is unbounded.
This will cause \sysname to overestimate model performance when using log loss as the performance metric.
In practice this should not be probelematic when the range is set sufficiently large.
