# Supplementary material for: Privacy Accounting and Quality Control in the Sage Differentially Private ML Platform
Source: arXiv:1909.01502 source file (2019-09-06)
Supplement: Supplementary file 4 [file private_trees.tex]

\begin{algorithm}
\begin{algorithmic}
\Procedure{PrivateSplit}{Training Data $X$, $\epsilon$ privacy budget, $\Theta$ splitting criteria}

    \For{$i = 0$ to $|\Theta|$}
        \State $I_i \leftarrow 0$ // initialize splitting criteria impurities to zero.
    \EndFor
    \For{$\theta_i \in \Theta$}
        \State // Compute the left partition average label.
        \State $X_l \leftarrow x_i \in X$ where $x_i[\theta_{item}] < \theta_{threshold}$
        \State $\text{avg}_l \leftarrow \frac{\sum{i \in X_l} y_i}{|X_l|}$.
        \State // Compute the right partition average label.
        \State $X_r \leftarrow x_i \in X$ where $x_i[\theta_{item}] \ge \theta_{threshold}$
        \State $\text{avg}_r \leftarrow \frac{\sum{i \in X_r} y_i}{|X_r|}$.
        \State // Compute the sum of squares error.
        \State $I_i \leftarrow \sum_{i \in X_r}(y_i - \text{avg}_r) ^ 2 + \sum_{i \in X_l}(y_i - \text{avg}_l) ^ 2$
    \EndFor
    \State // Choose the splitting criteria using the exponential
    \State // mechanism with sensitivity 1.
    \State return $\text{ExpMech}(I, 1, \epsilon)$
\EndProcedure

\Procedure{ComputeBudget}{$\epsilon$ privacy budget, maximum tree depth $m$, current depth $c$}
\State return $\frac{\epsilon}{2^{m-c}}$
\EndProcedure

\Procedure{PrivateBuildTree}{Training Data $X$ of size $n$, $\epsilon$ privacy budget, maximum tree depth $m$, current depth $c$, $\Theta$ splitting criteria}
    \State // Split the budget such that the lower levels are allocated more budget.
    \State $\hat{\epsilon} \leftarrow \frac{\epsilon}{2^{m-c+1}}$
    \If{$m = c$}
        \State // Assign remaining budget to the leaf.
        \State $\hat{\epsilon} \leftarrow \hat{\epsilon} + \frac{1.0}{2^{m+1}}$
        \State // Assign the node label.
        \State $\frac{\sum_{y_i \in X}{y_i} +\text{Laplace}(2/\hat{\epsilon})}{n + \text{Laplace}(2/\hat{\epsilon})}$
        \State return
    \EndIf
    \State $\theta \leftarrow PrivateSplit(X, \hat{\epsilon}, \Theta)$
    \State $X_l \leftarrow x_i \in X$ where $x_i[\theta_{\text{item}}] < \theta_{\text{threshold}}$
    \State $X_r \leftarrow x_i \in X$ where $x_i[\theta_{\text{item}}] \ge \theta_{\text{threshold}}$
    \State PrivateBuildTree($X_l$, $\epsilon$, $m$, $c+1$, $\Theta$)
    \State PrivateBuildTree($X_r$, $\epsilon$, $m$, $c+1$, $\Theta$)
\EndProcedure

\Procedure{PrivateBuildForest}{Training Data $X$ of size $n$, number of trees $t$, maximum tree depth $m$, $\Theta$ splitting criteria}
\State $\hat{\epsilon} \leftarrow \frac{\epsilon}{t}$
    \For{$i = 0$ to $t$}
        \State PrivateBuildTree($X$, $m$, $0$, $\hat{\epsilon}$)
    \EndFor
\EndProcedure
\end{algorithmic}
\caption{PrivateDecisionTrees.}
\label{alg:private_split}
\end{algorithm}
