# Supplementary material for: Privacy Accounting and Quality Control in the Sage Differentially Private ML Platform
Source: arXiv:1909.01502 source file (2019-09-06)
Supplement: Supplementary file 5 [file semantics.tex]

\subsection{Problem Definition}

\begin{figure}[t]
\centering
  \includegraphics[width=0.48\textwidth]{figures/block_stream.png}
  \vspace{-0pt}
  \caption{{\bf \sysname's setup.}
A stream of data split into blocks, forming a \blockstream, and used to run DP queries on
different subsets.
}
\label{fig:blockstream}
\end{figure}

We first need to define the guarantees we are targeting. At a high level, we
have a (infinite) dataset (or stream where we keep the history) partitioned in
block, and we want to perform Differentially Private (DP) queries on overlapping
subsets (defined by one or more blocks) of this dataset. We want the output of
these queries to be DP at the observation level with regards to the entire
dataset.

\paragraph{DP Background}

We now review useful definitions and prior results.

\definition{(Neighboring Datasets~\cite{Mcsherry:pinq}).}\label{def:neighboring}
We use the concept of neighboring datasets from~\cite{Mcsherry:pinq}. Viewing a
dataset as a multiset, we say that datasets $D$ and $D'$ are neighboring if
their symmetric difference (or disjunctive union, the elements which are in one
of the sets but not in their intersection) is at most one, noted $|D \oplus D'|
\leq 1$.

Intuitively this definition means that the attacker can add or remove a record
in the dataset, but changing a record corresponds to a symmetric difference of
size $2$, which can be supported using group
privacy~\cite{dwork2014algorithmic}. As in PINQ~\cite{Mcsherry:pinq}, we use
this definition as it is better adapted to the analysis of DP over splits of the
dataset. Changing one record can indeed affect two splits (is the key used for
the split changes), while adding or removing records affect only one split.

\definition{(Differential Privacy~\cite{dwork2014algorithmic}).}\label{def:dp}
A randomized mechanism $\M : \D \rightarrow \Y$ is $(\epsilon, \delta)$-Differentially Private if,
for all neighboring $\D$ and $\D'$, and for all $\ES \subseteq \Y$:
\[
  P(M(\D) \in S) \leq e^\epsilon P(M(\D') \in S) + \delta
\]

A common tool to analyse differential privacy is to define the Privacy Loss.
\definition{(Privacy Loss).}\label{def:privacy-loss}
For an outcome $y \in \Y$ and neighboring datasets $\D$ and $\D'$, the Privacy
Loss $Loss_\M(y; \D,\D')$ is defined as:
\[
  Loss_\M(y; \D,\D') = ln\Big( \frac{P(\M(\D) = y)}{P(\M(\D') = y)} \Big)
\]

Being able to bound the Privacy Loss for any neighboring datasets, with high probability over draws
$y \sim \M(\D)$ implies Differential Privacy.
\lemma{(\cite{kasiviswanathan2014semantics}).}\label{lemma:pl} If for all neighboring $\D$ and $\D'$, with probability
at least $(1 - \delta)$ over draws from $y \sim \M(\D)$, we have:
\[
  | Loss_\M(y; \D,\D') | \leq \epsilon ,
\]
then $\M$ is $(\epsilon, \delta)$-Differentially Private.

\paragraph{Block Stream Dataset}
Traditionally DP has been defined in the context of a
dataset~\cite{dwork2014algorithmic}. An algorithm can access any observation of
this dataset $\D$, and the privacy loss is thus accounted for at the level of
this dataset.
In \sysname however, new models are constantly trained on a stream of data, both
on subsets of past data and newly arrived observations. Fig.~\ref{fig:blockstream}
shows the setup.
If we were to use the traditional dataset paradigm, the privacy loss would
decrease at the whole stream level for each query, meaning that data not even
yet in the system would be impacted by training algorithms and no access would
be possible after the privacy budget is exhausted, even on future data.
\xxx{TODO (Mathias): explain why we want queries to overlap multiple blocks. E.g. histogram over feature, some small counts, we want to add noise only once over many blocks. Maybe: present as strawmens: regular accounting with stream is dataset. And split per block and treat as separate datasets.}
For instance, in Fig.~\ref{fig:blockstream}, if queries $Q1$ and $Q2$ exhaust
the privacy budget, $Q3$ cannot be performed although it queries a subset of the
data that was never seen before. Even worse, after block $H$ is collected, $Q4$
that queries only this new data cannot be performed either.
Intuitively, this is too conservative, as absent (or not queried) data cannot be
leaked by an algorithm. We need a different way to model the dataset to account
for privacy loss at a finer granularity, such that each query can discount privacy
budget only on the blocks they use. Moreover, we want to support overlapping queries.
For instance, if $Q1\text{-}4$ used only half of their blocks' budget, we want to be
able to perform $Q5$ on the remaining budget of each block.

To account for privacy loss at a finer granularity \sysname defines a
\blockstream: a sequence of data blocks $\D = (\D_1, \dots, \D_k)$, with a block
being the unit at which privacy loss is accounted for.  The block delimitation
is data independent (e.g. blocks correspond to a given time window).
We say that two \blockstream s $\D$ and $\D'$ are {\em adjacent} or {\em
neighboring} if there exists a block $k$ and index $i$ in block $k$ such that
$\D$ and $\D'$ differ only in observation $i$ in block $k$.
Formally, $\D_{l \neq k} = \D'_{l \neq k}$ and $|\D_{k} \oplus \D'_{k}| \leq 1$.
We note $\D_{(k)}$ and $\D'_{(k)}$ two neighboring \blockstream s that differ by
an observation in block $k$.
We next define how an adversary can interact with such a \blockstream~and show
how this enables block level privacy accounting.

\paragraph{Adversary Definition and Reduction To Block Level Privacy Loss}

In \sysname, we want to ensure differential privacy when training multiple models over time, on the \blockstream~$\D$. To formalize the power of an adversary $\A$ observing the trained models, and following~\cite{kairouz2015composition, rogers2016privacy}, we define the following composition game:

{\footnotesize
\begin{algorithm}
  \caption{BlockCompose($\A$, $b$, $r$), where $\A$ is a randomized algorithm, $b$ denotes two hypotheses of neighboring datasets, $r$ is the number of rounds.}
\begin{algorithmic}
  \State Select coin tosses $R^b_\A$ for $\A$ uniformly at random.
  \State $\A$ gives $k$, the block in which streams can differ (i.e. $\D^0_{l \neq k} = \D^1_{l \neq k}$ ; $|\D^0_{k} \oplus \D^1_{k}| \leq 1$).
  \For{$i$ in $1$, $\dots$, $r$}
    \State $\A = \A(\A^b_1, \dots, \A^b_i))$ gives neighboring datasets that differ in block $k$ $\D_{(k)}^{i,0}$ and $\D_{(k)}^{i,1}$, $(\epsilon_i, \delta_i)$-DP algorithm $\M_i$, and $blocks_i$ a subset of blocks from $\D_{(k)}^{i,b}$ to query.
    \State $\A$ receives $\A^b_i = \M_i(\bigcup\limits_{j \in blocks_i} \D_{(k),j}^{i,b})$, the result of running $\M_i$ on the subset $blocks_i$ of $\D_{(k)}^{i,b}$.
  \EndFor
  \Return{$V^b = (R^b_\A, \A^b_1, \dots, \A^b_r)$}
\end{algorithmic}
\label{algo:adacomp}
\end{algorithm}
}

At a high level, the adversary interacts with one of two adjacent datasets
($\D^0$ and $\D^1$) over multiple rounds. Each time the adversary submits a new
query that can depend on the previous results.  After receiving the result of
each query the adversary should not be able to distinguish between $\D^0$ and
$\D^1$.
We emphasize a number of important points in this composition game.
First, the neighboring \blockstream s are fixed over the while interaction game,
as opposed to previous composition theorems that support any neighboring
datasets at each round.  The setup of Algorithm \ref{algo:adacomp} is thus more
restrictive, but we believe closer to the use case of an adversary interacting
with a dataset, allowing us to account for privacy loss at the block level.
Second, the number of interactions $r$ is fixed in advance. However it will not
appear in the analysis and can thus be set to any extremely large number.

\definition{(Stream Level Privacy Loss).}\label{def:streamprivacyloss}
Call $v \sim V^b = (R^b_\A, \A^b_1, \dots, \A^b_r)$ a realization from $V^b$. The stream level privacy loss is the privacy loss considering the entire stream as dataset: $Loss_{\A}(v; \D^0,\D^1) = ln \Big( \prod\limits_{i=1}^r \frac{P(\A_i^0 = v_i | v_{<i})}{P(\A_i^1 = v_i | v_{<i})} \Big)$.

\definition{(Block Level Privacy Loss).}\label{def:blockprivacyloss}
We define the block level privacy loss for block $k$ as the privacy loss incurred from all queries computed on block $k$. Each query may also use data from other blocks. Formally, the block level privacy loss for block $k$ is defined as $Loss_{\A_{(k)}}(v; \D_{(k)}^0,\D_{(k)}^1) = ln \Big( \prod\limits_{\substack{i=1 \\ k \in blocks_i}}^r \frac{P(\A_i^0 = v_i | v_{<i})}{P(\A_i^1 = v_i | v_{<i})} \Big)$ the privacy loss for block $k$ counting only queries that use block $k$, that is for which $\{i, k \in block_i\}$.

\theorem{(Reduction to Block Level DP Composition).}\label{prop:reduction}
The privacy loss under the composition game from Algorithm \ref{algo:adacomp} is
upper-bounded by the maximum privacy loss for any given block:
\begin{align*}
  &  \forall \A, \forall (\D^0, \D^1): \\
  &  | Loss_\A(v; \D^0,\D^1) | \leq \max_{i} | Loss_{\A_{(i)}}(v; \D_{(i)}^0,\D_{(i)}^1) | .
\end{align*}
\begin{proof}
We note $v_i$ the $i^{th}$ element of $v$, and $v_{<i}$ all elements preceding
the $i^{th}$.  We first show that for a fixed $k$, the stream privacy loss
is the block privacy loss for block $k$:
\begin{align*}
  \big| & Loss_\A(v; \D_{(k)}^0,\D_{(k)}^1) \big| = \big| ln \Big( \prod_{i=1}^r \frac{P(\A_i^0 = v_i | v_{<i})}{P(\A_i^1 = v_i | v_{<i})} \Big) \big| \\
   & = \big| ln \Big( \prod_{\substack{i=1 \\ k \in blocks_i}}^r \frac{P(\A_i^0 = v_i | v_{<i})}{P(\A_i^1 = v_i | v_{<i})} \Big) \\
   & ~ \ ~ + ln \Big( \prod_{\substack{i=1 \\ k \notin blocks_i}}^r \frac{P(\A_i^0 = v_i | v_{<i})}{P(\A_i^1 = v_i | v_{<i})} \Big) \big| \\
   & = \big| Loss_{\A_{(k)}}(v; \D_{(k)}^0,\D_{(k)}^1) \big| ,
\end{align*}
  because if $k \notin blocks_i$, then $\bigcup\limits_{j \in blocks_i} \D_{(k),j}^{0} = \bigcup\limits_{j \in blocks_i} \D_{(k),j}^{1}$ and thus $\frac{P(\A_i^0 = v_i | v_{<i})}{P(\A_i^1 =v_i | v_{<i})} = 1$.

We can now bound the privacy loss against any adversary $\A$ in Algorithm
\ref{algo:adacomp} for any $(\D^0, \D^1)$:
\begin{align*}
  \forall (\D^0, \D^1), \exists k \ \text{s.t.} \ \D^0_{l \neq k} & = \D^1_{l \neq k} \ \text{and} \ |\D^0_{k} \oplus \D^1_{k}| \leq 1:\\
  \big| Loss_\A(v; \D^0,\D^1) \big| & = \big| Loss_{\A_{(k)}}(v; \D_{(k)}^0,\D_{(k)}^1) \big| \\
                                    & \leq \max_{i} \big| Loss_{\A_{(i)}}(v; \D_{(i)}^0,\D_{(i)}^1) \big| ,
\end{align*}
which concludes the proof.
\end{proof}

In other words, the privacy loss can be accounted for at the block level.

\paragraph{Composition}
\label{sec:adacomp}

Because multiple models are continuously trained is \sysname, we need to account for the composition
of multiple queries on the \blockstream.
Theorem~\ref{prop:reduction} directly yields a result for basic composition.
\theorem{(Basic Composition for Block Stream Datasets).}\label{prop:basiccomp}
If $|Loss_{\M_i}(v_i, D^0, D^1; v_{<i})| \leq \epsilon_i(v_{<i})$ with probability at least $1-\delta_i(v_{<i})$ (implying that $\M_i$ is $(\epsilon_i(v_{<i}), \delta_i(v_{<i}))$-DP) then for any ($\D^0,\D^1$) and any adversary $\A$ in Algorithm \ref{algo:adacomp}, with probability at least $1-(\max_i \sum\limits_{j \in blocks_i} \delta_j)$:
\begin{align*}
  & | Loss_\A(v; \D^0,\D^1) | \leq \max_{i} \sum\limits_{j \in blocks_i} \epsilon_j ,
\end{align*}
making $\A$ $(\epsilon, \delta)$-DP with $\epsilon = \max_{i} \sum\limits_{j \in
blocks_i} \epsilon_j$ and $\delta = \sum\limits_{j \in blocks_i} \delta_j$ from Lemma~\ref{lemma:pl}.
\begin{proof}
We follow the proof from Theorem~\ref{prop:reduction}:
\begin{align*}
\end{align*}
\end{proof}
In other words, the DP parameters sum per block, and the algorithm is DP with
regards to the whole stream with the worse block-wise parameters. Note that the
DP parameters for each query $(\epsilon_i(v_{<i}), \delta_i(v_{<i}))$ depend on
past results and are themselves random variables. For simple composition (i.e.
``summing epsilons and deltas'') the composition result is not impacted. This
result was already observed in~\cite{rogers2016privacy} and holds when $\M_i$ is
$(\epsilon_i, \delta_i)$-DP --a slightly weaker condition than the high
probability bound on the privacy loss-- although the proof is more complicated.

When a large number of queries are performed however, which we would expect in
\sysname's setting, it is advantageous to use so-called strong composition
theorems, as in practice the privacy loss can be more tightly bounded that with
basic composition. In this case, having DP parameters that depend on the history
is more problematic, as is prevents us from using typical strong composition
theorems~\cite{}. The only to remove this dependency and use strong composition
would be to declare in advance for every query both their DP parameters and the
blocks that will be queried. This is not compatible with \sysname's use-case of
reclaiming unused privacy budgets and aggregating it over multiple blocks to train
new models.

{\footnotesize
\begin{algorithm*}[t]
  \caption{BlockFilterCompose($\A$, $b$, $r$, $\epsilon_g$, $\delta_g$), where $\A$ is a randomized algorithm, $b$ denotes two hypotheses of neighboring datasets, $r$ is the number of rounds, $(\epsilon_g,\delta_g)$ the global privacy parameters to enforce.}
\begin{algorithmic}
  \State Select coin tosses $R^b_\A$ for $\A$ uniformly at random.
  \State $\A$ gives $k$, the block in which streams can differ (i.e. $\D^0_{l \neq k} = \D^1_{l \neq k}$ ; $|\D^0_{k} \oplus \D^1_{k}| \leq 1$).
  \For{$i$ in $1$, $\dots$, $r$}
    \State $\A = \A(\A^b_1, \dots, \A^b_i))$ gives neighboring datasets that differ in block $k$ $\D_{(k)}^{i,0}$ and $\D_{(k)}^{i,1}$, $(\epsilon_i, \delta_i)$-DP algorithm $\M_i$, and $blocks_i$ a subset of blocks from $\D_{(k)}^{i,b}$ to query.
    \If{$\exists k \in blocks_i, FILT^k_{\epsilon_g,\delta_g}(\epsilon_1, \delta_1, ..., \epsilon_i, \delta_i, 0, 0, ...) = HALT$}
      \State $(\A_i,...,\A_r) = \perp$
      \State BREAK
    \Else
      \State $\A$ receives $\A^b_i = \M_i(\bigcup\limits_{j \in blocks_i} \D_{(k),j}^{i,b})$, the result of running $\M_i$ on the subset $blocks_i$ of $\D_{(k)}^{i,b}$.
    \EndIf
  \EndFor
  \Return{$V^b = (R^b_\A, \A^b_1, \dots, \A^b_r)$}
\end{algorithmic}
\label{algo:adacomp}
\end{algorithm*}
}

We thus leverage privacy filters~\cite{rogers2016privacy}, designed to provide...
We could also use an odometer.

We make important remarks to highlight the flexibility of this scheme:
Early stopping is allowed and $r$ does not play a role in the analysis, so the number of rounds is not a limitation.
Since choosing the blocks adaptively already requires adaptive privacy parameters, they can be fully adaptive.
