# Supplementary material for: Privacy Accounting and Quality Control in the Sage Differentially Private ML Platform
Source: arXiv:1909.01502 source file (2019-09-06)
Supplement: Supplementary file 6 [file appendix.tex]

\section{PTK Profiling Proofs}
\label{appendix:profiling-proofs}
